# Supplementary material for: CLIP: A Dataset for Extracting Action Items for Physicians from Hospital Discharge Notes
Source: arXiv:2106.02524 source file (2021-06-04)
Supplement: Supplementary file 1 [file appendix.tex]

\appendix

\begin{figure*}[t]
  \centering 
  \includegraphics[scale=0.7]{figures/table_1_image.png}
  \caption{Example of a highlighted discharge summary (a public sample from United Health Network). }
  \label{fig:highlighted_summary_2} 
\end{figure*}
